# Supplementary material for: Post-Training Quantization for 3D Medical Image Segmentation: A Practical Study on Real Inference Engines
Source: arXiv:2501.17343 source file (2025-01-28)
Supplement: Supplementary file 1 [file appendix.tex]

\newcolumntype{x}[1]{>{\centering\arraybackslash}p{#1pt}}
\newcolumntype{z}[1]{>{\raggedright\arraybackslash}p{#1pt}}

\newpage
\clearpage
\section*{Appendix: CLIP-Driven Universal Model}
\appendix

%\title{Supplementary for CLIP-Driven Universal Model for Organ Segmentation and Tumor Detection}
%\maketitle
% \begin{spacing}{1.30}  \centering \LARGE  \bf{Supplementary Materials for \\ CLIP-Driven Universal Model} \end{spacing}

\noindent\textbf{Abstract.} In this supplementary material, we provide additional information about
